# Supplementary material for: Raman Spectra of Titanium Carbide MXene from Machine-Learning Force Field Molecular Dynamics
Source: arXiv:2209.15294 source file (2022-09-30)
Supplement: Supplementary file 1 [file SI.pdf]

# Supporting Information: Raman Spectra of Titanium Carbide MXene from Machine-Learning Force Field Molecular Dynamics

Ethan Berger,[*,†] Zhong-Peng Lv,[‡] and Hannu-Pekka Komsa[*,†]

†*Microelectronics Research Unit, Faculty of Information Technology and Electrical Engineering, University of Oulu, P.O. Box 4500, Oulu, FIN-90014, Finland*

‡*Department of Applied Physics, Aalto University, Aalto, FIN-00076, Finland*

E-mail: ethan.berger@oulu.fi; hannu-pekka.komsa@oulu.fi

## Synthesis and Raman measurement of $Ti_3C_2T_x$

An aqueous dispersion of $Ti_3C_2T_x$ was synthesized using MILD method.[1] In a typical recipe, 2 g $Ti_3AlC_2$ (325 mesh, Carbon-Ukraine) was gradually added to a mixture of 40 mL 9 M HCl and 2 g LiF at 35 °C. After stirring for 24 h, the product was centrifuged and washed with deionized water until pH was above 5. Then, 40 mL of water was added to the sediment and vortexed for 30 min. The mixture was centrifuged at 3500 rpm for 30 min to obtain the supernatant containing few-layered $Ti_3C_2T_x$ and then stored at 4 °C in $N_2$ atmosphere. The $Ti_3C_2T_x$ concentration was determined by weighting the dried self-standing film filtrated from a certain volume of the $Ti_3C_2T_x$ dispersion.

The Raman spectrum of $Ti_3C_2T_x$ was performed on the Horiba Jobin-Yvon confocal Raman system. For Raman sample preparation, the $Ti_3C_2T_x$ dispersion was first diluted to 0.1 mg mL$^{-1}$. Then 5 $\mu$L of the diluted dispersion was drop-casted on a $1\times1$ cm$^2$ highly ordered pyrolytic graphite (HOPG) substrate pre-treated with 5 min of $O_2$ plasma. The Raman spectrum was acquired from few-layer $Ti_3C_2T_x$ flakes under 60 s exposure time of 15 mW 785 nm semiconductor laser with $\times100$ objective.

## Resonant Raman spectra

Since $Ti_3C_2T_x$ is metallic, the measured Raman spectra is always under resonant conditions. The effect of the excitation wavelength on the spectra has already been studied experimentally, showing little impact on peaks other than the titanium mode at 120 cm$^{-1}$.[2] Fig. S1 shows resonant Raman spectra for different excitation wavelength. In particular, Fig. S1(a) shows results obtained using the Raman tensors of the pure oxygen unit cell. Peak intensities are fairly sensitive to the choice of laser wavelength. At 516 nm, the spectrum shows all peaks that are observed in experiments, even though the $A_{1g}(T_x)$ mode at 300-400 cm$^{-1}$ seem dominant and its intensity overestimated. Similar remark can be made when using the Raman tensors and eigenvectors of the pure -OH unit cell, represented in Fig. S1(b). In this case, the peak intensities all seem equal, in particular at 516 nm,

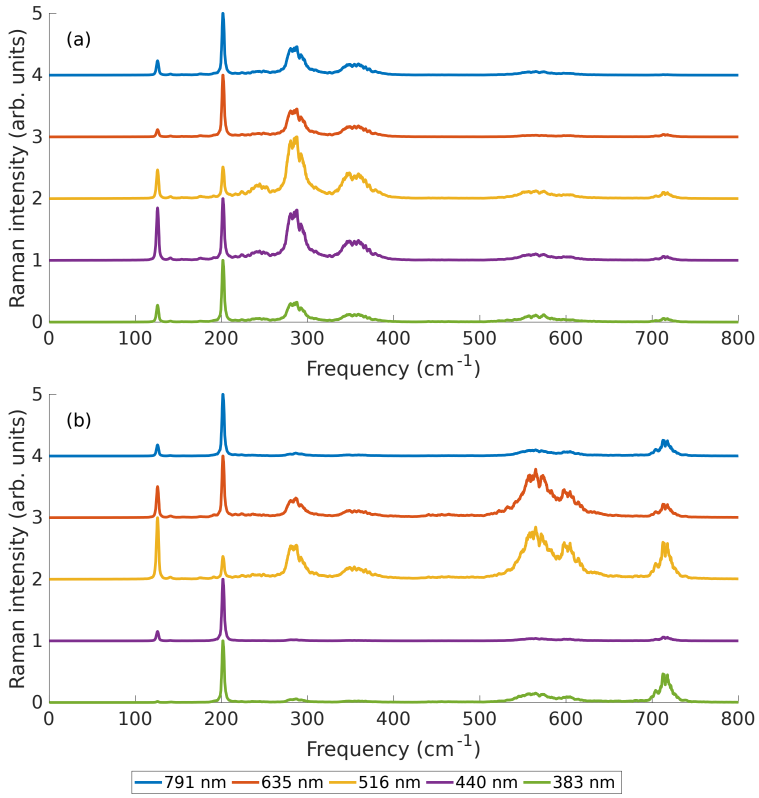


Figure S1: Resonant Raman at different excitation wavelengths from RGDOS using (a) pure oxygen and (b) pure -OH eigenvectors and Raman tensors. The wavelengths are labeled at the bottom.

which is in good agreement with experimental measurements (see Fig. 1 for example). However, our results differ from the experimental ones at frequencies other than 516 nm. Indeed, while experiments show little impact of the excitation energy on the peaks intensities, our calculation indicate the opposite. One explanation could be that we are using Raman tensors of pure surfaces unit cells. In this case, some peaks might be active only at some precise wavelengths, since the dielectric function and its change with displacement can display sharp features. On the other hand, in the case of mixed surfaces, it is expected that the dielectric function (and its change with displacement) becomes broadened/smeared out. This ultimately leads to the excitation energy having less impact on the peak intensities, as observed in experiments where surfaces are mixed. This shows one of the limitation of RGDOS where we cannot use Raman tensors of systems with mixed surface. Note however that inaccuracies in the Raman tensors only impacts the intensities of the peaks, but do not change results concerning the width of the peaks. In this work, we will use Raman tensors of the pure -OH unit cell with an excitation wavelength of 516 nm.

# Comparison of distributions

To reduce the noise in the spectra shown in Figs. 4 and 5 of the main paper, we performed five MD runs for each concentration, with a different distribution of surface terminations in each run. Fig. S2 shows the Raman spectra from each run of $x = 0.5$ separately. All curves show similar peaks and thus we can safely average them. We note that the MLFF training is only performed for one distribution. Changing the distribution does not impact the MLFF accuracy and the resulting Raman spectra, so we can safely assume that the model correctly predicts other distributions as well as other concentrations.

# Lorentzian fitting of the peaks

In order to compare the frequencies of the peaks with experiments, we have to fit the peaks. We use a lorentzian function, as written in equation S1, where $a$ is the intensity, $\omega$ is the frequency, and

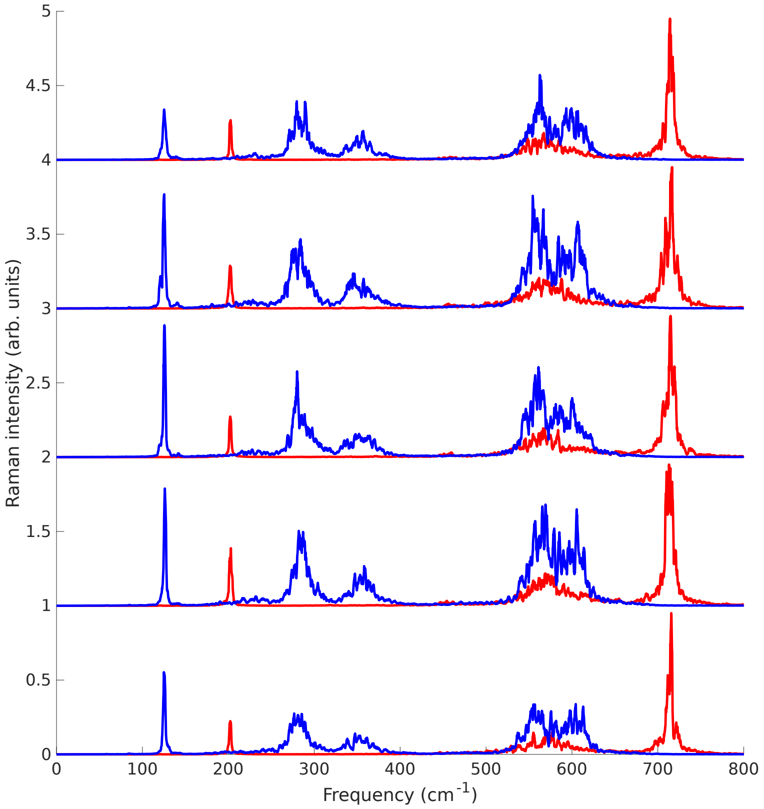


Figure S2: Raman spectra for x=0.5 concentration but different distributions of the surface terminations.

$G$ is the width of the peak. One of the interesting features of RGDOS is that the peaks can easily be isolated by only considering spectra projected to a particular eigenmode. Figs. S3 (a)-(c) show the $E_g$(Ti) and $A_{1g}$(Ti) modes as well as the $A_{1g}$(C) mode for different concentrations of surface terminations. The Lorentzian function nicely fits the spectra and the evolution of the frequencies can easily be followed. Numerical values of the frequencies are reported in Table 1 of the main article.

$$L(x) = \frac{a}{(x-\omega)^2 + (G/2)^2}. \tag{S1}$$

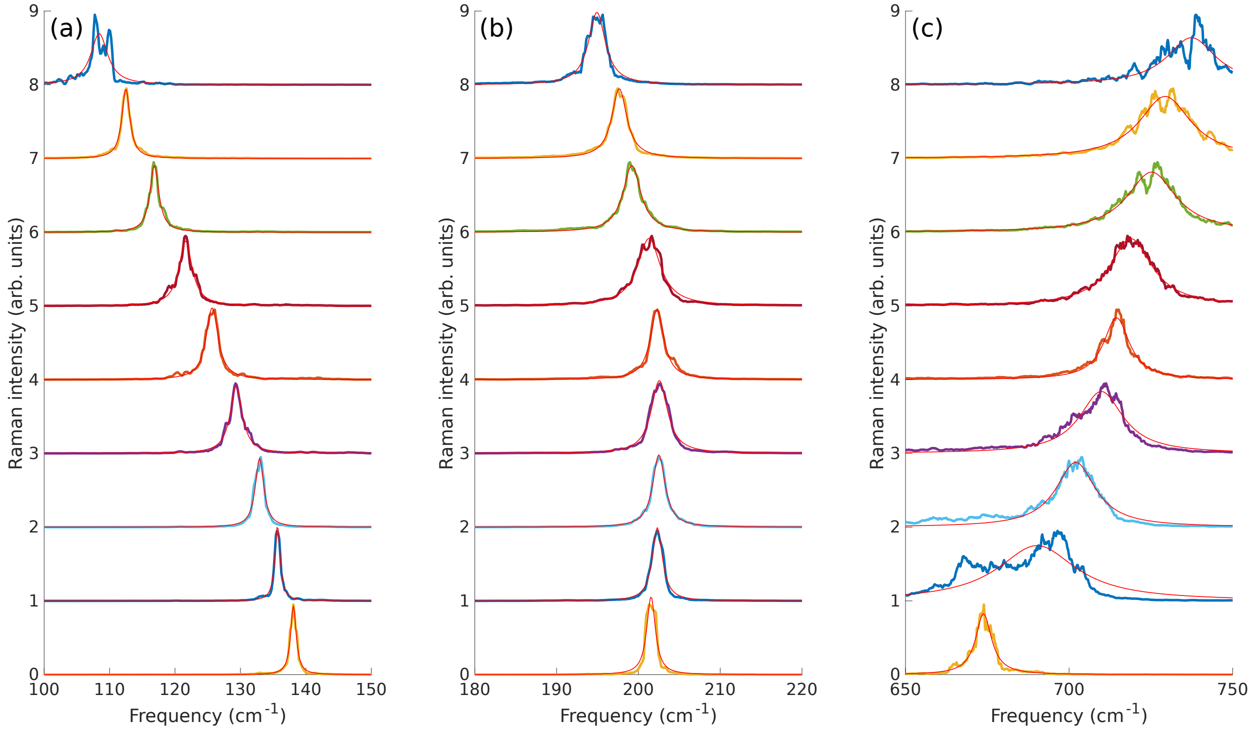


Figure S3: Isolated RDGOS peak of (a) the $E_g$(Ti) mode, (b) the $A_{1g}$(Ti) mode and (c) the $A_{1g}$(C) mode. The red lines represent Lorentzian fit of the peaks.

# Effect of multilayer and surface water.

To explain the wide peaks observed at 300–400 and 600 cm$^{-1}$, we investigated the effect of multilayer MXene and interaction with water molecules at the surface on the Raman spectra.

MLFF model is first extended to multilayer MXene by adding bulk and bilayer configurations. Bulk and bilayer structures were constructed from the monolayer and using a O-H-O chain to link the layers, which should be energetically the most favorable configuration at x=0.5.[3] Note that two different stacking configurations were studied for the bulk phase. Both converged to the ideal configuration where O-H-O are aligned between layers during the training MD. Production runs were therefore started from this stacking for bulk phase and multilayers. Results for different number of layers and bulk MXene are shown in Fig. S4(a). While the transition from monolayer to bulk shows clear changes, there are no sign of wide peaks. We conclude that multilayer is not responsible for the widening of peaks.

MLFF model is then extended to describe water molecules at the MXene surface. The model is trained by adding small amount of molecules (2 in the beginning) at the surface and progressively increasing this number (up to 10 molecules). Note that all of the water molecules are located on the same surface for both training and production MDs. Results for various number of molecules are shown in Fig. S4(b). Overall, water molecules seem to have fairly little impact on the Raman spectra and again do not explain the wide features observed in experiments.

## Phonon density of states

To observe the effect of modes outside $\Gamma$-point on the Raman spectra, we study the phonon density of states obtained from velocity auto-correlation function (VACF).

The total phonon DOS from VACF is shown in Fig. S5(a), but cannot be directly compared to experiments since it also contains the Raman-inactive modes. Fig. S5(b) shows the VACF projected on the Raman active modes only and decomposed into contributions from each mode.

To better reproduce the Raman spectra, one can keep only the contribution from the Raman active modes and sum over the first Brillouin zone using the weights shown in Fig. 5(b). Such results are represented in Fig. S6 for every concentrations and in Fig. 5(c) of the main paper for the x=0.5 concentration. The resulting spectra are in good agreement with the experimental results.

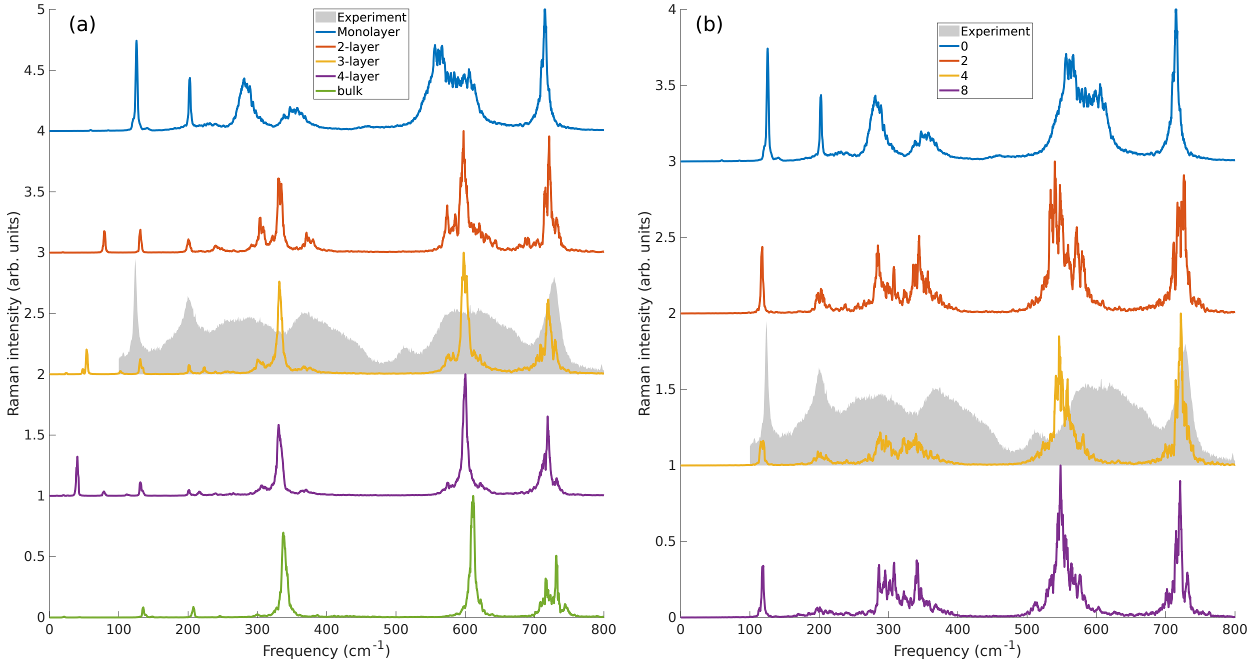


Figure S4: (a) Raman spectra for monolayer, multilayer and bulk MXene. (b) Raman spectra of MXene with different number of water molecules interacting at the surface.

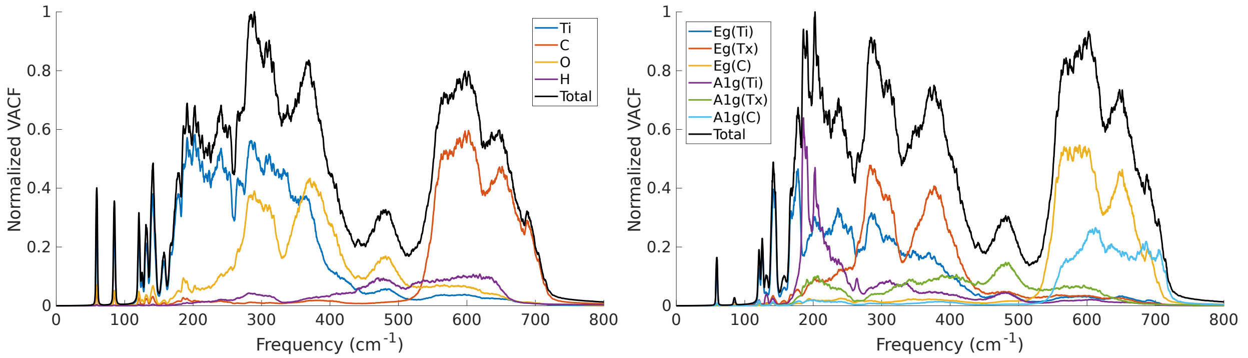


Figure S5: (a) Total phonon density of states from VACF for $x = 0.5$. (b) VACF projected onto the Raman active modes. Contributions from each Raman active modes are also shown.

In particular, there is finally an agreement for the large widths of peaks in the 300–400 $cm^{-1}$ and 600 $cm^{-1}$. These peaks remain in good agreement for different surface compositions, showing the minor impact of surface concentration on these peaks.

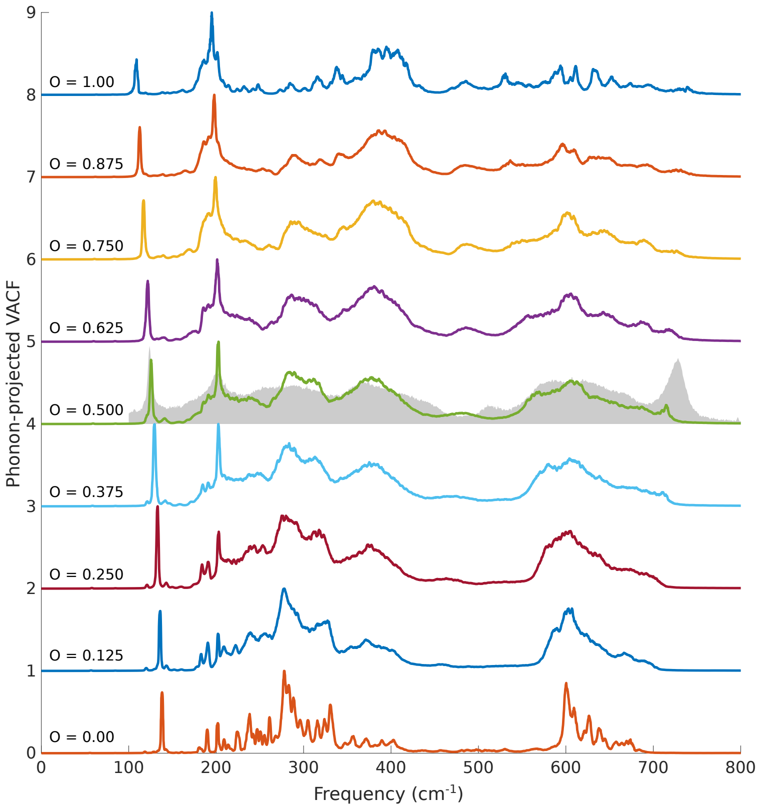


Figure S6: Weighted phonon-projected VACF of Raman active modes for different concentrations of surface concentrations.

# References


(1) Alhabeb, M.; Maleski, K.; Anasori, B.; Lelyukh, P.; Clark, L.; Sin, S.; Gogotsi, Y. Guidelines for Synthesis and Processing of Two-Dimensional Titanium Carbide (Ti 3 C 2 T x MXene). *Chemistry of Materials* **2017**, *29*, 7633–7644.

(2) Sarycheva, A.; Gogotsi, Y. Raman Spectroscopy Analysis of the Structure and Surface Chemistry of Ti3C2Tx MXene. *Chemistry of Materials* **2020**, *32*, 3480–3488.

(3) Hu, T.; Hu, M.; Li, Z.; Zhang, H.; Zhang, C.; Wang, J.; Wang, X. Interlayer coupling in two-dimensional titanium carbide MXenes. *Phys. Chem. Chem. Phys.* **2016**, *18*, 20256–20260.
